# Supplementary material for: Ensuring Solution Uniqueness in Fixed-Point-Based Harmonic Power Flow Analysis with Converter-Interfaced Resources: Ex-post Conditions
Source: arXiv:2403.12595 source file (2024-03-19)
Supplement: Supplementary file 1 [file Appendix3.tex]

\begin{equation*}\label{eq:72}
     \frac{\partial}{\partial \hat{W}_\rho}\hat{W}_{{k,R}} = \left[\begin{array}{ccccccccc}
     \left[
     \begin{array}{cc}
         -\dfrac{P_{\sigma}}{v^2_{\gamma,D,0}} & 0  \\
         \dfrac{Q_{\sigma}}{v^2_{\gamma,D,0}} & 0
     \end{array}\right] & &  & & 
       \left[
     \begin{array}{cc}
         2\dfrac{v_{\gamma,D,-26}}{v^3_{\gamma,D,0}}P_{\sigma}  & 0 \\
         -2\dfrac{v_{\gamma,D,-26}}{v^3_{\gamma,D,0}}Q_\sigma  & 0
     \end{array}\right] & \\
     &    \left[
     \begin{array}{cc}
         -\dfrac{P_{\sigma}}{v^2_{\gamma,D,0}} & 0\\
         \dfrac{Q_{\sigma}}{v^2_{\gamma,D,0}} & 0
     \end{array}\right] & &  &\left[
     \begin{array}{cc}
         2\dfrac{v_{\gamma,D,-25}}{v^3_{\gamma,D,0}}P_{\sigma}& 0  \\
         -2\dfrac{v_{\gamma,D,-25}}{v^3_{\gamma,D,0}}Q_\sigma  & 0
     \end{array}\right]\\
     & & \ddots & &\vdots & \\
     & & & &\left[
     \begin{array}{cc}
         -\dfrac{P_{\sigma}}{v^2_{\gamma,D,0}} & 0 \\
         \dfrac{Q_{\sigma}}{v^2_{\gamma,D,0}} & 0
     \end{array}\right] \\
     & & & & \left[ \begin{array}{cc}
         2\dfrac{v_{\gamma,D,1}}{v^3_{\gamma,D,0}}P_{\sigma} & 0 \\
         -2\dfrac{v_{\gamma,D,1}}{v^3_{\gamma,D,0}}Q_\sigma  & 0
     \end{array}\right] & \left[
     \begin{array}{cc}
         -\dfrac{P_{\sigma}}{v^2_{\gamma,D,0}}  & 0\\
         \dfrac{Q_{\sigma}}{v^2_{\gamma,D,0}} & 0
     \end{array}\right]\\
     & & & & \vdots & &\ddots \\

     \end{array}\right]
\end{equation*}

\subsection{Recall from grid-following CIDER model library}
\begin{equation}
    \mathbf{w}_\kappa(t) = \mathbf{i}^*_{\gamma,\text{DQ}}(t)
\end{equation}

\begin{equation}
    \mathbf{i}^*_{\gamma,\text{DQ}}(t) = \frac{1}{v_{\gamma,\text{D}}(t)}\left[\begin{array}{c}
         P_\sigma  \\
         -Q_\sigma 
    \end{array}\right]
\end{equation}
\begin{equation}
    w_\rho = v_{\gamma,\text{D}}(t)
\end{equation}
\begin{equation}
    \frac{1}{v_{\gamma,\text{D}}(t)} \approx \frac{1}{v_{\gamma,\text{D,0}}}\left(1-\xi_{\text{D}}(t)+\xi_{\text{D}}^2(t)\right)
\end{equation}
\begin{equation}
    \frac{1}{v_{\gamma,\text{D}}(t)} \approx \sum_h \Psi_h \exp{(jh2\pi f_1t)}
\end{equation}

\begin{equation}
    \hat{W}_{\text{k},R}(\hat{W}_\rho,S_\sigma) \approx \left[\begin{array}{cc}
         -\dfrac{v_{\gamma,D,-26}}{v^2_{\gamma,D,0}}P_{\sigma}  \\
        \dfrac{v_{\gamma,D,-26}}{v^2_{\gamma,D,0}}Q_{\sigma} \\
        \vdots \\
        \dfrac{1}{v_{\gamma,D,0}}P_{\sigma}  \\
        -\dfrac{1}{v_{\gamma,D,0}}Q_{\sigma} \\
        \vdots \\
        -\dfrac{v_{\gamma,D,26}}{v^2_{\gamma,D,0}}P_{\sigma}  \\
        \dfrac{v_{\gamma,D,26}}{v^2_{\gamma,D,0}}Q_{\sigma} \\
    \end{array}
    \right]\quad \text{and} \quad 
       W_\rho = \left[  
    \begin{array}{c}
         v_{\gamma,D,-26}  \\
         v_{\gamma,Q,-26} \\
        \vdots \\
        v_{\gamma,D,0}  \\
         v_{\gamma,Q,0} \\
        \vdots \\
        v_{\gamma,D,26}  \\
         v_{\gamma,Q,26} \\
    \end{array}
    \right]
\end{equation}
