# Supplementary material for: Ensuring Solution Uniqueness in Fixed-Point-Based Harmonic Power Flow Analysis with Converter-Interfaced Resources: Ex-post Conditions
Source: arXiv:2403.12595 source file (2024-03-19)
Supplement: Supplementary file 2 [file Appendix2.tex]

\section{Linear Time Periodic Systems}\label{sec:Appendix2}
\begin{equation}
    \mathbf{A}(t)\mathbf{x}(t) \leftrightarrow \mathbf{A}(f)\ast\mathbf{X}(f) = \hat{\mathbf{A}}\hat{\mathbf{X}}
\end{equation}
